# Supplementary material for: Similar Part Rearrangement With Pebble Graphs
Source: arXiv:1404.6573 source file (2014-04-25)
Supplement: Supplementary file 1 [file 08_appendix.tex]

\subsection{Proof of Near Optimality}

Let there be $m$ stablized states in $V_{elite}$, e.g. $X_{c} = \{x_0, x_1, ..., x_m\}$, where $m<N(R_p, X_{free})$. $X_{m}$ is the ``claimed regions'' which is consist of $m$ ball regions centered at each stablized state. Let {\tt Interior}($X_m$) denote the set of all interior states, {\tt Surface}($X_m$) denote the set of all surface states, and {\tt Exterior}($X_m$) denote the set of all exterior states.

\begin{lemmma}
Let $x$ be a state such that $x\in {\tt Interior}(X_m)$ and $x\neq x_i$, where $0\leq i\leq m$. Then $x$ does not exist.
\end{lemmma}

Since Lemma[Uniqueness in Each Ball], the above Lemma is immediate.

\begin{lemmma}
Let $x$ be a state such that $x\in {\tt Exterior}(X_m)$. Then there must exist a state $x^\prime$ such that (i) $x^\prime\in{\tt Surface}(X_m)$; and (ii) {\tt Cost}($x^\prime$) $<$ {\tt Cost}($x$).
\end{lemmma}

The above Lemma is trivial since the trajectory starting from $x_0$ to $x$ must go through {\tt Surface}($X_m$). And since the cost function is {\tt Additive} and {\tt Non-negative}, the lemma holds.

Let $x^\ast_{m+1}$ be a state in {\tt Surface}($X_m$) and such that for any $x^\prime_{m+1}\in{\tt Surface}(X_m)$ and $x^\prime_{m+1}\neq x^\ast_{m+1}$, there is {\tt Cost}($x^\ast_{m+1}$) $\leq$ {\tt Cost}($x^\prime_{m+1}$). There could be several $x^\ast_{m+1}$. Obviously they all have the same cost. Let $X^\ast_{m+1}$ denote the set of all $x^\ast_{m+1}$.

\begin{thm}
\emph{[Growth of Stablized Region]} Given infinite iterations, there must be a new stablized state $x_{m+1}\in V_{elite}$ and $x_{m+1}\in X^\ast_{m+1}$.
\end{thm}

The above theorm holds since Lemma[Non-diminishing Positive Change] and Assumption[Completeness of Random Shooting], given infinite iterations, all states in ${\tt Surface}(X_m)$ will be reached with optimal edges starting from $X_{m}$. And since Lemma 8 and Lemma 9, states in $X^\ast_{m+1}$ must have the smallest cost. They must have been reached and the {\tt Drain} function never put them out of $V_{elite}$. Therefore, one of the $x^\ast_{m+1}$ must be the next stablized state after $x_{m}$.

Given Lemma[Start Region Exclusivity], Lemma[Finite Number of Balls], and Theorm[Growth of Stablized Region], the next Lemma is immediate.

\begin{lemmma}
Given infinite iterations, $V_{elite}$ contains and only contains all $N(R_p, X_{free})$ stablized states.
\end{lemmma}

There are some interesting properties for stablized states.

\begin{lemmma}
\emph{[Optimal Wavefront]} Let $x_i$ and $x_j$ be two stablized states and $x_i$ is discovered earlier than $x_j$, so $i<j$. There must be that {\tt}Cost($x_i$) $\leq$ {\tt}Cost($x_j$).
\end{lemmma}

The above Lemma comes from Lemma[Non-Negative] and Lemma[Additive]. Since {\tt}Cost($x_i$) = {\tt Min}\{{\tt Cost}({\tt Surface}($X_{i-l}$))\} and {\tt}Cost($x_j$) = {\tt Min}\{{\tt Cost}({\tt Surface}($X_{i+l}$))\}, where $l=j-i-1$. {\tt Cost}({\tt Surface}($X_m$)) is non-decreasing. The surface regions behave like a wavefront propagating from the low cost regions to high cost regions.

\begin{lemmma}
\emph{[Convergence to $RRT^\ast$ Edges]} Given infinite iterations, $E_{\rrtdrain}^\infty(V)=E_{{\tt RRT}^*}^N(V)$
\end{lemmma}

According to percolation theroy, stablized state $x_i$ has $K$ nearest neighbor states. There are $K$ edges from neighbors to $x_i$, denoted as $E_{in}$. And there are $K$ edges from $x_i$ to neighbors, denoted as $E_{out}$. When $x_i$ is inserted in $V_{elite}$, the algorithm only generated a subset of edges, denoted as $E_{in}^{prev}$, which consists of the neighbors that are already in $X_{i-1}$. The rest of the edges are from stablized states after $x_i$ to $x_i$. They are more costly according to Lemma[Optimal Wavefront]. The algorithm keeps the edge $e_{in}^\ast$ in $E_{in}^{prev}$ that results in the minimum cost at $x_i$. $e_{in}^\ast$ is also the edge in $E_{in}$ to contribute to the mininum cost at $x_i$. On the other hand, when inserting stablized states that are after $x_i$, a subset of edges in $E_{out}$ are generated, denoted as $E_{out}^{next}$. These edges are taken care of when inserting neighbors after $x_i$. $E_{out}^{prev}$ are edges from $x_i$ to the neighbors before $x_i$. They are not generated when these neighbors are inserted. However, they are not necessary since they will not contribute to best connection according to Lemma[Optimal Wavefront]. Therefore, Lemma[Convergence to $RRT^\ast$ Edges] holds.

Given Lemma 11 and Lemma 13, if $RRT^\ast$ has the same set of vertices at iteration $N(R_p,X_{free})$, theorm[Near Optimality] holds.

\subsection{Proof of Deterministic Reachability}

\begin{lemmma}
${\tt Surface}(X_{N(R_p,X_{free})})\cap X_{reachable}\cap X_{free}=\emptyset$
\end{lemmma}

According to theorm[Growth of Stablized Region], as long as {\tt Surface}($X_{m}$) in the collision-free reachable region is not {\tt empty} set, there will be a new stablized state $x_{m+1}$ given infinite iterations. And since there are at most $N(R_p,X_{free})$ stablized states, there must be that {\tt Surface}($X_{N(R_p,X_{free})}$) in the collision-free reachable region is empty set. 

\begin{lemmma}
${\tt Exterior}(X_{N(R_p,X_{free})})\cap X_{reachable}\cap X_{free}=\emptyset$
\end{lemmma}

Given Lemma 14, according to the definition of $exterior$ $regions$, the above Lemma must hold.

Given Lemma 15, according to the definition of $interior$ $regions$, the theorm[Deterministical Reachability] must hold.
